# Supplementary material for: Benchmarking Psychological Dynamics in Generative Agents
Source: arXiv:2610.04246 source file (2026-10-03)
Supplement: Supplementary file 1 [file appendix.tex]

\appendix

\section{Within-Person Magnitude: Sources of Compression and Routes to Recovery}
\label{app:magnitude}

The benchmark recovers the direction of within-person relations while their magnitude stays close to
zero. This appendix seeks to explicate why a generative rater returns a small, central deviation when a larger
one fits the day, a pattern we term the safe-deviation tendency, and reports the levers that enlarge it.
We separate routes available to an all-silico evaluation from routes that require longitudinal human data.

\subsection{The safe-deviation tendency}
\label{app:safe}

Several mechanisms push a rater toward a timid, central response.

\textbf{The rating is a conditional mean.} Asked for an end-of-day state, the model reports its
expectation over plausible responses, which is smoother than a single sampled realization of the
underlying process. The reported series therefore carries less within-person variance than the latent
state it represents. The near-deterministic ratings we observe, with single-rating reliability
\relYMean{}, indicate that the rater commits to this expectation, which is also why the within-person
correlation holds at \withinRtempEight{} under rating temperature 0.8 and \withinRtempZero{} under
temperature 0.0.

\textbf{Alignment rewards the modal answer.} Instruction tuning and preference optimization favor
moderate, broadly acceptable outputs and discourage commitment to scale extremes, so the rater settles
toward the middle of each range. The capability pattern in Section~\ref{app:capability} makes this
concrete: general capability and within-person recovery move in opposite directions.

\textbf{The supplied baseline acts as a prior.} Providing the rater its own trait baseline and typical
range invites shrinkage toward that prior, compressing each day toward the persona average. Removing the
anchor sharpens directional recovery, with sign agreement rising from \dirFull{} to \dirDeanchor{} and
rank correlation from \rhoFull{} to \rhoDeanchor{}, while the magnitude holds steady. Anchoring is
therefore one contributing cause among several.

\textbf{Signal weakens across two mappings.} A day's drivers pass from seeded indicators to narrative
and from narrative to rating. Each mapping regresses toward its own central tendency, so the covariation
between an indicator and the state it should move arrives at measurement after two rounds of smoothing.

The combined result is a rater that identifies the correct sign of a day's effect and renders it as a
small, safe deviation: faithful in direction, timid in magnitude.

\subsection{Capability and within-person recovery}
\label{app:capability}

Holding the prompt and the data fixed, we re-rated the shared narratives with three models that span the
gpt-4.1 family. As capability falls, the within-person rank signal strengthens: rank correlation against
meta-analytic effects rises from \rhoFull{} for gpt-4.1, through \miniRho{} for gpt-4.1-mini, to
\nanoRho{} for gpt-4.1-nano, and sign agreement reaches \nanoDir{} for the smallest model. The magnitude
stays near the sampling floor across the whole ladder, between \withinRbaseline{} and 0.028. The reading
is that the lighter-aligned model preserves the day-to-day variation that the structure requires, while
the magnitude remains governed by the construct's variance budget rather than by model capability.

\subsection{Construct variance and within-person recovery}
\label{app:icc}

The variance budget is set by the intraclass correlation. The four headline states are trait-saturated,
with ICC near 0.75, so the within-person share available for any indicator to move is small. We tested
three constructs with a more even between- and within-person split by re-rating the same narratives for
daily exhaustion (ICC \exhaustICC{}), fatigue (ICC \fatigueICC{}), and flow (ICC \flowICC{}). Within-person
magnitude rises in step with the within-person variance share: pooled $|r|$ reaches \exhaustWithinR{} for
exhaustion, \fatigueWithinR{} for fatigue, and \flowWithinR{} for flow, roughly three times the
\withinRbaseline{} of the trait-saturated set, with sign agreement of \exhaustDir{} and \fatigueDir{} and
rank correlation up to \fatigueRho{}. These estimates rest on \nIccPairs{} anchored pairs per state and
serve as a directional demonstration. The pattern locates the magnitude limit in the construct rather
than in the model: where a state carries real day-to-day variance, the synthetic population reproduces
within-person structure at a size the literature recognizes.

\subsection{In-silico achievability of the structural targets}
\label{app:achieve}

A complementary question is whether the structural targets are reachable by optimization using
published norms alone, holding measured human states out of the objective entirely. We optimized the
rating prompt with MIPROv2 against a literature-only objective: the within-person standard deviation
implied by published ICC values, use of the full scale range, avoidance of ceiling and floor pileup, and
the cross-state coherence band on the \nVerifiedL{} verified meta-analytic pairs. Optimization ran on
\nTuneTrain{} training personas, and we report the composite on \nTuneTest{} personas kept aside from
optimization. The tuned prompt raises the held-out composite from \miniBaseComp{} to \miniTunedComp{} for
gpt-4.1-mini and from \nanoBaseComp{} to \nanoTunedComp{} for gpt-4.1-nano. The gains are small and
consistent, which places the uniform off-the-shelf prompt already close to the in-silico ceiling for
these targets while confirming that optimization against published norms yields a measurable structural
improvement on held-out data. The instruction the optimizer selected encodes the same anti-anchoring move
identified in Section~\ref{app:safe}: it directs the rater to let the texture of the day move each rating
toward the ends of its scale. These results establish reachability on a fully all-silico footing, distinct
from the question of predicting realized individual trajectories.

\subsection{A principled bound and the routes that remain}
\label{app:bound}

Two readings follow. First, the magnitude ceiling is structural: when between-person variance dominates,
the recoverable within-person correlation is bounded, and a timid magnitude on trait-saturated states is
the expected outcome. Second, the routes that raise magnitude on an all-silico footing act on variance
and structure: a lighter-aligned rater (Section~\ref{app:capability}), constructs with a larger
within-person share (Section~\ref{app:icc}), de-anchored rating, and narratives that encode the day's
drivers more vividly. Routes that condition on an individual's measured history, namely personalized
exemplars, neighbor retrieval, and fitted statistical predictors, raise pooled coefficients while their
within-person component stays near chance, and they depend on measured human states; they belong to the
companion problem of predicting realized individual trajectories. The honest target for an all-silico
benchmark is the fidelity of within-person variance, range, and direction against published effects, with
magnitude reported as a construct-bounded quantity.
